# Supplementary material for: Coupled dynamics of long-range and internal spin cluster order in Cu$_{2}$OSeO$_{3}$
Source: arXiv:1902.05329 ancillary file (2019-02-14)
Supplement: Supplementary file 1 [file CoupledDynamicsSupplMat.pdf]

# Supplementary Information: Coupled dynamics of long-range and internal spin cluster order in $Cu_2OSeO_3$

Rolf B. Versteeg,[1] Jingyi Zhu,[1] Christoph Boguschewski,[1] Fumiya Sekiguchi,[1] Anuja Sahasrabudhe,[1] Kestutis Budzinauskas,[1] Prashant Padmanabhan,[1] Petra Becker,[2] Daniel I. Khomskii,[1] and Paul H. M. van Loosdrecht[1]

[1]*Institute of Physics 2, Faculty of Mathematics and Natural Sciences, University of Cologne, Zülpicher Straße 77, D-50937 Cologne, Germany*

[2]*Institute of Geology and Mineralogy, Faculty of Mathematics and Natural Sciences, University of Cologne, Zülpicher Straße 49b, D-50674 Cologne, Germany*

The long timescale spin-lattice equilibration is microscopically dictated by the coupling between acoustic phonons, and low- and high-energy spin cluster excitations. We fitted a phenomenological three temperature model[1] (3TM) to the 10's to 100's ps-decade dynamics transients in order to obtain the disordering time for the long-range and internal spin cluster order. We consider a closed system after $t > 6$ ps, with effective temperatures $T_{\mathrm{acoustic}}{=}T_{\mathrm{ac.}}$ for the acoustic phonon bath, $T_{\mathrm{low-E}}$ for the low-energy spin cluster excitation bath, and $T_{\mathrm{high-E}}$ for the high-energy spin cluster excitation bath.

From the high-energy spin excitation peak shift at $t = 850$ ps we deduce a quasi-equilibrium temperature $\Delta T \approx 7$ K above $T_{\mathrm{bias}} = 5$ K, i.e. T(850 ps) ≈ 12 K. The acoustic phonon temperature, indicated with blue spheres in Fig. 4 of the main article, is linearly proportional to the recovery of the 103 meV phonon scattering intensity, with $T_{\mathrm{acoustic}}(850\,\mathrm{ps}) \approx 12$ K and $T_{\mathrm{acoustic}}(6\,\mathrm{ps}) \approx 14$ K. The high-energy spin excitation temperature, indicated with orange spheres, is linearly proportional to the increasing component of the transient spin excitation spectral weight transfer $SW$. The quasi-equilibrium temperature is set to $T_{\mathrm{high-E}} \approx 12$ K. The temperature at $t = 6$ ps is set to about $T_{\mathrm{low-E}} \approx 5.5$ K, i.e. slightly above $T_{\mathrm{bias}} = 5$ K.

The three-temperature model is given as follows:

$$\begin{aligned} C_{\mathrm{ac.}} \frac{\partial T_{\mathrm{ac.}}}{\partial t} &= -g_1(T_{\mathrm{ac.}} - T_{\mathrm{low-E}}) - g_2(T_{\mathrm{ac.}} - T_{\mathrm{high-E}}) \\ C_{\mathrm{low-E}} \frac{\partial T_{\mathrm{low-E}}}{\partial t} &= -g_1(T_{\mathrm{low-E}} - T_{\mathrm{ac.}}) - g_3(T_{\mathrm{low-E}} - T_{\mathrm{high-E}}) \\ C_{\mathrm{high-E}} \frac{\partial T_{\mathrm{high-E}}}{\partial t} &= -g_2(T_{\mathrm{high-E}} - T_{\mathrm{ac.}}) - g_3(T_{\mathrm{high-E}} - T_{\mathrm{low-E}}) \end{aligned} \qquad (1)$$

where the $C_i$'s indicate the heat capacities of the respective quasiparticle baths, and the $g_i$'s their couplings. To be more specific: $g_1 \equiv g_{\mathrm{ac.-low-E}}$, $g_2 \equiv g_{\mathrm{ac.-high-E}}$, and $g_3 \equiv g_{\mathrm{low-E-high-E}}$. The (relative) heat capacities for the acoustic phonon, low-energy spin excitation and high-energy spin excitation baths are set to fulfill $C_{\mathrm{acoustic}} > C_{\mathrm{low-E}} \gg C_{\mathrm{high-E}}$ $(1 > 0.25 > 5 \cdot 10^{-8})$ (Ref. 2). The difference between the temperature transients $T_{\mathrm{acoustic}}$ and $T_{\mathrm{high-E}}$ and their respective 3TM functions are minimized by varying the coupling parameters $g_i$. The resulting temperature functions are plotted with solid lines in Fig. 4 of the main manuscript.

$T_{\mathrm{low-E}}$ approximately exponentially increases with $\tau_{\mathrm{LRO}} \sim 55$ ps, giving the long-range disordering time. The high-energy spin excitations form a dual probe of long-range and internal spin cluster order. Assuming a bi-exponential decay for the high-energy spin excitation transient, we find a $\tau_{\mathrm{cluster}} \sim 400$ ps for the disordering of internal spin cluster order.

[1] A. Kirilyuk, A. V. Kimel, and T. Rasing, Ultrafast optical manipulation of magnetic order, Rev. Mod. Phys. **82**, 2731 (2010).

[2] N. Prasai, B. A. Trump, G. G. Marcus, A. Akopyan, S. X. Huang, T. M. McQueen, and J. L. Cohn, Ballistic magnon heat conduction and possible Poiseuille flow in the helimagnetic insulator $Cu_2OSeO_3$, Phys. Rev. B **95**, 224407 (2017).
